# Supplementary material for: Enhanced physics-constrained deep neural networks for modeling vanadium redox flow battery
Source: arXiv:2203.01985 source file (2022-03-03)
Supplement: Supplementary file 1 [file appendix.tex]

%%%%%%%%%%%%%%%%%%%%%%%%%%%%
%%% appendix %%%
%%%%%%%%%%%%%%%%%%%%%%%%%%%%
\appendix

%%% ---------------------------------
% 0D models
%%% ---------------------------------
\section{Analytical solution of species concentrations}\label{sec:append-concentration}
%
Following the 0D model proposed in \cite{Shah2011}, the species considered in the reaction kinetics are $\mathcal{S} = \{\text{V(II)}, \text{V(III)}, \text{V(IV)}, \text{V(V)}, \text{H}^+, \text{H}_2 \text{O}\}$. 
Let $c_i^{res}$ and $c_i$ be the concentrations of species $i$ ($ i \in \mathcal{S}$) in the reservoir and the electrode, respectively. Note that both $c_i^{res}$ and $c_i$ are space-independent functions due to the assumption of uniform distribution in the 0D model.
Thus, the recirculation of the electrolytes through reservoris changes the concentrations of all species in the electrodes together with electrochemical reaction.

With a uniform flow rate at the inlet, the net change per unit time ($\text{mol/s}$) of species $i$ in the electrode due to recirculation is approximately equal to $\epsilon A_{in} u ( c_i^{res} - c_i)$, where $\epsilon$ is the porosity of the electrode, $u$ is the electrolyte flow velocity (in $\text{m/s}$), and $A_{in} = b_e w_e$ is the inlet area of the electrode, in which $b_e$ and $w_e$ are the breadth and width, respectively (see Fig. \ref{fig:sche_model} and the default values given in Table \ref{table:ex1_model}). Here, we define $\tilde{u} = \epsilon u =  \omega /A_{in}$ as the average velocity in the porous medium, where $\omega$ is the inlet volume flow rate. Therefore, the mass conservation of species $i$ in the reservoris is:
\begin{equation}\label{eq:mass_res}
	V_r \frac{d c_i^{res}}{dt} = - A_{in} \tilde{u} ( c_i^{res} - c_i)
	%= - \frac{\epsilon \delta u}{h_e} ( c_i^{res} - c_i), \quad i \in \mathcal{S}
\end{equation}
where $V_r$ is the volume of the reservoir.


In the electrodes, we introduce the electrochemical reaction in addition to the recirculation, and the mass balance for species ($i = \text{V(II), V(III), V(IV), V(V)}$)  are expressed as follows:
\begin{subequations}\label{eq:mass_ele}
	\begin{align}
		& \epsilon V_e \frac{d c_i}{dt} = A_{in} \tilde{u} ( c_i^{res} - c_i) - \frac{I}{F}, \quad i = \text{V(II), V(V)} \\
		& \epsilon V_e \frac{d c_i}{dt} = A_{in} \tilde{u} ( c_i^{res} - c_i) + \frac{I}{F}, \quad i = \text{V(III), V(IV)}
	\end{align}
\end{subequations}
%\begin{equation}\label{eq:kine_v2}
%\epsilon V_e \frac{d c_i}{dt} = A_{in} \tilde{u} ( c_i^{res} - c_i) - \frac{I}{F}, \quad i = V(II), V(V)
%\end{equation}
%\begin{equation}\label{eq:kine_v3}
%\epsilon V_e \frac{d c_i}{dt} = \epsilon A_{in} u ( c_i^{res} - c_i) + A_s \frac{j_{app}}{F}, \quad i = \text{V(III), V(IV)}
%\end{equation}
where $I$ is the applied current, $V_e = b_e w_e h_e$ is the volume of the electrode, and $h_e$ is the length of the electrode. Eliminating the recirculation terms in Eqs. (\ref{eq:mass_res}) and (\ref{eq:mass_ele}) and performing integration with using the initial conditions $c_i = c_i^{res} = c_i^0$, the solutions of electrode concentrations can be obtained:
\begin{subequations}\label{eq:soln_ele}
	\begin{align}
		& c_i = c_i^0 - \frac{I}{V_e F \epsilon \tilde{ \epsilon} } \left(\frac{\epsilon \delta + e^{-\tilde{ \epsilon} t}}{1+ \epsilon \delta} - 1 - \frac{\epsilon \delta}{\tau} t \right), \quad i = \text{V(II), V(V)} \\
		& c_i = c_i^0 + \frac{I}{V_e F \epsilon \tilde{ \epsilon}} \left(\frac{\epsilon \delta + e^{-\tilde{ \epsilon} t}}{1+ \epsilon \delta} - 1 - \frac{\epsilon \delta}{\tau} t \right), \quad i = \text{V(III), V(IV)}
	\end{align}
\end{subequations}
where $\delta = V_e/V_r$ is the ratio of the two volumes, $\tau = h_e/u$ and $\tilde{\epsilon} = (\epsilon \delta + 1)/\tau$. With the concentration of vanadium specifies, the state of charge (SOC) \cite{You2009a} is defined as
% An important factor of the charge or discharge process is State of Charge (SOC) which introduces the amount of electrochemical energy stored in the tanks, and is described as follows:
%\begin{equation}\label{eq:soc}
%\text{SOC}(t) = \frac{c_{\text{V(II)}}(t)}{c_{V_n}^0} = \frac{c_{\text{V(V)}}(t)}{c_{V_p}^0}
%\end{equation}
\begin{equation}\label{eq:soc}
	\text{SOC}(t) = \frac{c_{\text{V(II)}}(t)}{c_{V_n}^0} = 1 -  \frac{c_{\text{V(III)}}(t)}{c_{V_n}^0}
\end{equation}
where $c_{V_n}^0$ is the initial vanadium concentration of the negative half-cell. Given $c_{\text{V(III)}}^0 = c_{V_n}^0$ and substituting the analytical solution of $c_{\text{V(III)}}$ in Eq. (\ref{eq:soln_ele}b) into Eq. (\ref{eq:soc}), SOC can be rewritten as
\begin{equation}\label{eq:soc_t}
	\text{SOC}(t) = - \frac{I}{c_{V_n}^0 V_e F \epsilon \tilde{ \epsilon} } \left(\frac{\epsilon \delta + e^{-\tilde{ \epsilon} t}}{1+ \epsilon \delta} - 1 - \frac{\epsilon \delta}{\tau} t \right)
\end{equation}
The SOC estimated by Eq. (\ref{eq:soc}) and (\ref{eq:soc_t}) is used as a input varibale in the proposed PINN framework introduced in Section \ref{sec:pinn}.

A similar procedure is adopted for the concentrations of water and protons, i.e. $c_{\text{H}_2 \text{O}}$ and $c_{\text{H}^+}$.  Considering the recirculation,  electrochemical reaction, and osmotic drag effect, the mass conservation of water is
\begin{subequations}\label{eq:mass_water}
	\begin{align} 
		%	c_{\text{H}_2 \text{O}}
		& - \text{ve electrode}: \epsilon V_e \frac{d c_{\text{H}_2 \text{O}}}{dt} = A_{in} \tilde{u} ( c_{\text{H}_2 \text{O}}^{res} - c_{\text{H}_2 \text{O}}) + \frac{ n_d I}{F}  \\
		& + \text{ve electrode}: \epsilon V_e \frac{d c_{\text{H}_2 \text{O}}}{dt} = A_{in} \tilde{u}  ( c_{\text{H}_2 \text{O}}^{res} - c_{\text{H}_2 \text{O}}) -  \frac{(1+ n_d) I}{F}
	\end{align}
\end{subequations}
Herein, the molar flux of water through the membrane from the positive to negative electrode during charging is approximated by $n_d j_{app}/F$, where $n_d$ is the drage coefficent, $j_{app} = I/A_e$ is the nominal current density, and $A_e = h_e w_e$ is the electrode area. By using the mass balance equation in (\ref{eq:mass_res}) with $i = \text{H}_2 \text{O}$ to eliminate the recirculation terms, the solution to Eq. (\ref{eq:mass_water}) reads
\begin{subequations}\label{eq:soln_water}
	\begin{align}
		& - \text{ve electrode}:  c_{\text{H}_2 \text{O}} = c_{\text{H}_2 \text{O}}^0 
		- \frac{I n_d}{V_e F \epsilon \tilde{ \epsilon} }
		\left(\frac{\epsilon \delta + e^{-\tilde{ \epsilon} t}}{1+ \epsilon \delta} - 1 - \frac{\epsilon \delta}{\tau} t \right)\\
		& +\text{ve electrode}: c_{\text{H}_2 \text{O}} = c_{\text{H}_2 \text{O}}^0 
		+ \frac{I}{V_e F \epsilon \tilde{ \epsilon}} (1+n_d)
		\left(\frac{\epsilon \delta + e^{-\tilde{ \epsilon} t}}{1+ \epsilon \delta} - 1 - \frac{\epsilon \delta}{\tau} t \right)
	\end{align}
\end{subequations}
Relating to the SOC in Eq. (\ref{eq:soc_t}), the water concentration in the positive electrode $c_{\text{H}_2 \text{O}_p}$ is expressed as: $c_{\text{H}_2 \text{O}_p} = c_{\text{H}_2 \text{O}_p}^0 - c_{V_n}^0 \times \text{SOC}$. The mass balance for the protons are:
\begin{subequations}\label{eq:mass_proton}
	\begin{align} 
		%	\text{H}+
		& - \text{ve electrode}: \epsilon V_e \frac{d c_{\text{H}^+}}{dt} = A_{in} \tilde{u} ( c_{\text{H}^+}^{res} - c_{\text{H}^+}) + \frac{I}{F}  \\
		& + \text{ve electrode}: \epsilon V_e \frac{d c_{\text{H}^+}}{dt} = A_{in} \tilde{u}  ( c_{\text{H}^+}^{res} - c_{\text{H}^+}) +  \frac{I}{F}
	\end{align}
\end{subequations}
For simplicity, in the above equaiton (\ref{eq:mass_proton}) we assume a rapid transport of protons across the fully saturated membrane such that the protons are evenly distributed in both postive and negative electrodes, which is different from the original formulation in \cite{Shah2011}. 
Thus, the proton concentrations in both electrodes are:
\begin{equation}\label{eq:soln_proton}
	c_{\text{H}^+} = c_{\text{H}^{+}}^0
	- \frac{I}{V_e F \epsilon \tilde{ \epsilon} }
	\left(\frac{\epsilon \delta + e^{-\tilde{ \epsilon} t}}{1+ \epsilon \delta} - 1 - \frac{\epsilon \delta}{\tau} t \right)
\end{equation}
or expressed as $c_{\text{H}^+} = c_{\text{H}^{+}}^0 + c_{V_n}^0 \times \text{SOC}$.
%- \text{ve electrode} \text{and}  + \text{ve electrode}:

%The model parameters used for the equaitons in this section can be referred to \textcolor{blue}{Table []}.
%Note that in the above equations, the specifice surface area and the drag coefficient for osmotic drag are usually fitted parameters. The membrane is asssumed to be fully saturated such that the proton molecures pass through membrane with maximun capacity. In addition, $\epsilon A_{in} u$ is defined as the flow rate $\omega$.

% [2014_Chen Yeoh]
%\textit{The assumptions and simplifications used by Vynnycky [33] are adopted in the present model unless otherwise stated. Briefly, the major assumptions are pseudo steady state isothermal opera- tion, dilute-solution approximation, electroneutrality in the bulk, full ionization of the excess sulphuric acid as supporting elec- trolyte, negligible electromigration, plug-flow for the circulating electrolyte, negligible trans-membrane water migration, and neg- ligible side reactions. 
%The constant concentration assumption will be relaxed to account for the varying concentrations of all active species on two fronts: first, changes in the bulk compared to the inlet; and second, between the bulk and the surface of the electrodes. These con- centration differences will become prominent when the VRFB is operated at low electrolyte flow rates and at high current densities [17,18].}
%
%% Proton [2014_Chen Yeoh]
%\textit{Although protons are involved in the redox reaction at the positive half-cell as indicated by reaction (2), this model does not account for the differences between the bulk and the surface concentrations of protons for two reasons. Firstly, its bulk concen- tration is far more than that of the vanadium species in the anolyte, hence the proton is not the limiting reactant. Secondly, the diffusion coefficient of the proton is much higher than that of other species due to its hopping mechanism via water molecules [37], and as such any concentration gradient is expected to be smaller.}
