# Supplementary material for: Enhanced physics-constrained deep neural networks for modeling vanadium redox flow battery
Source: arXiv:2203.01985 source file (2022-03-03)
Supplement: Supplementary file 2 [file sec-supplement.tex]

% Assumption

\begin{enumerate}
	\item Only consider the species: $\mathcal{S}$ = \{V(II), V(III), V(IV), V(V), \ce{H+}, \ce{H2O}\}.
	\item All chemicals are distributed uniformly in the solute and instantaneous mixing with negligible reaction in the electrolyte tanks.
	\item The applied charge/discharge current is constant.
	\item Incompressible fluid.
	\item Membrane is assumed to be fully saturated with no accumulation.
	\item Cell potential is composed of the reversible voltage, and the activation and ohmic losses.
	\item Consier temperature effects
\end{enumerate}

% 2020 Choi
\textit{For the VRFB cell shown in Fig. 1 (b), the governing equations and relevant physical parameters are summarized in Table 1. Further, the source terms in the transport and charge convection equations are listed in Table 2. Here, we assumed a quasi-steady state [19] for the model, and isothermal and isotropic properties for the membrane and electrode; further we assumed the electrolyte as a dilute solution with electro- neutrality, negligible electromigration in the transport equations, no side reactions and crossover through the membrane, and plug flow in the porous electrode [18]. }
 
% surface density
 Differences between bulk and surface concentrations
 Due to the mass transport resistance from the bulk solution to the surface of the porous carbon electrode, the concentrations of the vanadium species on the surface of the porous electrode (cis) are (4) often different from those (ci) in the bulk.
 
 Key reference:
 [1] S. B. Lee et al., “Open data, models, and codes for vanadium redox batch cell systems: A systems approach using zero-dimensional models,” J. Electrochem. Energy Convers. Storage, vol. 17, no. 1, 2019.



%
It is well known that the accurate parameter estimation is critical to closely predict system behavior in the operting domain~\cite{0D,2D,3D,...}.
However, it remains difficult especially for the electrochemical models that are not directly observed.
\textit{[Wang (2018)] Published studies in chemical process parameter estimation are usually based on one of two types of data; either from laboratory data or pilot plant scale runs...}

In this study, we proposed a new methodology based on deep neural networks to estimate multiple electrochemical parameters. 

\textit{In this study, we propose to use physics-informed neural networks (PINNs) to identify the model parameter with respect to various operting conditions of the VRFB system. 
	For demonstration, we consider the inlet velocity $\tilde{u}$, applied current $I$, and the initial concentration }
\textcolor{blue}{In code, we use $\tilde{u}$}

\textit{I. Kroner, M. Becker, and T. Turek, “Determination of Rate Constants and Reaction Orders of Vanadium-Ion Kinetics on Carbon Fiber Electrodes.,” ChemElectroChem, no. September, 2020.}
Measuring correct Kinect data on porous electrodes is challenging for several reasons. 
•	First, it is difficult to estimate the real electrochemically active electrode surface area, which is additionally also varying due to changes in the manufacturing process. 
Wu and Holze[10] have outlined in their detailed review on catalysts for VFB how important the correct consideration of the active surface area is and introduced the term “true electrochemically active surface area” (EASA). In general, the EASA is calculated using the roughness of the electrode and its geometric surface area. Many studies use methods such as Brunauer-Emmet-Teller (BET) to determine the specific surface area of the electrode.[11]
•	In addition, the carbon material itself shows strong irregularities and varies in structure and reactivity.[10] The real electrochemi- cally active surface area should therefore be better determined by measuring the double-layer capacity with electrochemical impedance spectroscopy (EIS) or cyclic voltammetry (CV).[12]


\subsection{Disscussion: Limitations}
XXX.
(Shah, 2008): be aware the different between the draft effect and liquid-pressure gradients for water concentration
The model predicts a net transfer of water from the negative to positive electrode during charge (the net effect of the migration of hydrated protons and transport due to concentration and pressure gradients). During discharge the net transfer is initially from the negative to positive electrode but towards the end of the cycle reverses direction. (Important)

From Fig. 6(a) and (b) it appears that drag of water from the positive to negative electrode is not the domi- nant mechanism of transport, but rather back diffusion, which is caused by the developing concentration and liquid-pressure gra- dients from the negative to positive electrode. The magnitude of the drag coefficient depends on the current density, which in this example is low.



of interest, profiles of concentration, overpotential and current den- sity, as in Figs. 3–6. In situ experimental measurements of these quantities are extremely difficult to obtain, and in some cases impossible, yet this information (such as the likelihood of local- ized reactant depletion or of a steep potential rise) can be of vital importance to ensuring both good performance and longevity of the battery. To serve as a predictive tool the model would of course require extensive validation and possibly the inclusion of additional physical phenomena.


%%% ---------------------------------
% Example: I
%%% ---------------------------------
\subsection{Parameter identification for a small VRFB cell with different operating conditions}\label{sec:results_cfd2d}
Herein, we apply the PINN method to identify multiple model parameters $\vec{\mu}$ in the 0D numerical model for a small VRFB cell experiement considered in \cite{Shah2008}. 

For carefully examinate the learned parameter map, we generate a 64 2D simulation resuts using~\cite{Shah2008}...

Herein, we present material and model parameters used in the nu- merical simulation. In the cases where experimental methods were not feasible, numerical fitting is used to determine the parameters and the extracted values are compared to the peer-reviewed literature. Unless otherwise stated, all model and material parameters are listed in Tables 3–5 with references for the parameters given in the Ref. column, where the abbreviations exp., mfr., and est. refer to experiment, manufacturer, and estimated, respectively
